# Supplementary material for: Towards Personalized and Human-in-the-Loop Document Summarization
Source: arXiv:2108.09443 source file (2021-10-01)
Supplement: Supplementary file 1 [file chap_appendix.tex]

\chapter{An Appendix}

This is an appendix.  Add anything in here that you need in an appendix.
